# Supplementary material for: Buckling of a monolayer of plate-like particles trapped at a fluid-fluid interface
Source: arXiv:2307.01087 source file (2023-07-03)
Supplement: Supplementary file 1 [file appendix.tex]

\section{Interface shape}
The Fourier transform of equation (\ref{eqn:young_laplace}) with respect to $x$ is given as,

\begin{equation}
    -q^2 H + \frac{\partial^2 H}{\partial z^2} = \frac{H}{L_c^2}, \label{eqn:ode1}
\end{equation}

Where, $H$ is given as, 
\begin{align}
    H(q,z) = \mathcal{F} \left[ h(x,z)  \right] =\frac{1}{\sqrt{2 \pi}} \int_{- \infty}^{\infty} h(x,z) e^{i q x} dx 
\end{align}

Equation A12 is rewritten as follows, 

\begin{align}
    \frac{\partial^2 H}{\partial z^2} - (q^2 + \frac{1}{l_c^2}) H = 0
\end{align}
 
Here $H$ is a function of $q,z$ and it has a solution of the form, 

\begin{align}
\label{eqn:ans1}
    H = C e^{z\sqrt{q^2 + \frac{1}{l_c^2}}} + D e^{-z\sqrt{q^2 + \frac{1}{l_c^2}}}
\end{align}

To substitute the boundary conditions they have to expressed in the Fourier transform with respect to $q$. Given as,

\begin{align}
  h(x,z=\infty) &= 0  \\
  \mathcal{F} \left[ h(x,z=\infty)  \right] &= 0 \\
  H(q,z=\infty) &= 0 
\end{align}

Substituting this boundary condition in equation A15 gives C = 0. The other boundary condition is at the edge of the plates is,

\begin{align}
    h(x, z = 0) &= A \sin \left( \frac{2 \pi x}{\lambda}\right) \\
    \mathcal{F} \left[ h(x,z=0)  \right] &= H(q,z=0) \\
    =& i A \sqrt{\frac{\pi}{2}} \left[  \delta (q- 2\pi/\lambda) - \delta (q+2\pi/\lambda )  \right]
\end{align}
Substituting this boundary condition in equation A15,

\begin{align*}
    D = i A  \sqrt{\frac{\pi}{2}} \left[  \delta (q- 2\pi/\lambda) -  \delta (q+2\pi/\lambda )  \right ]
\end{align*}

Then,

\begin{align*}
    H(q,z) = i A \sqrt{\frac{\pi}{2}} \left[  \delta (q- 2\pi/\lambda) -  \delta (q+2\pi/\lambda )  \right ]  e^{-z\sqrt{q^2 + \frac{1}{l_c^2}}}
\end{align*}

And the shape of the interface is obtained by inverse Fourier transform of $H$ with respect to $q$, given as,

\begin{align}
    h(x,z) = \mathcal{F}^{-1} (H) &= \frac{1}{\sqrt{2 \pi}} \int_{-\infty}^{\infty} H(q,z) \ e^{-iqx}  dq
\end{align}

\begin{align*}
    h(x,z) &= \frac{1}{\sqrt{2 \pi}} i A \sqrt{\frac{\pi}{2}} \bigg \{ \int_{-\infty}^{\infty} \delta (q- 2\pi/\lambda) e^{-z\sqrt{q^2 + \frac{1}{l_c^2}}} e^{-iqx}  dq \\
    &- \int_{-\infty}^{\infty} \delta (q+ 2\pi/\lambda) e^{-z\sqrt{q^2 + \frac{1}{l_c^2}}} e^{-iqx}  dq  \bigg \}
\end{align*}
 
Simplifying this,
 
 \begin{align}
     %y(x,z) &= i \frac{4A}{\pi^2} \left\{  e^{-z\sqrt{(2\pi/\lambda)^2 + \frac{1}{L_c^2}}} e^{-i(2\pi/\lambda)x} - e^{-z\sqrt{(-2\pi/\lambda)^2 + \frac{1}{L_c^2}}} e^{-i(-2\pi/\lambda)x} \right\} \\
    h(x,z) &= i \frac{4A}{\pi^2} e^{-z\sqrt{(2\pi/\lambda)^2 + \frac{1}{l_c^2}}} \left \{  e^{-i(2\pi/\lambda)x} -   e^{i(2\pi/\lambda)x}  \right \} \\
     &=  i \frac{4A}{\pi^2} e^{-z\sqrt{(2\pi/\lambda)^2 + \frac{1}{l_c^2}}} (-2 i \sin ((2 \pi/\lambda)x) \\
     &=  A e^{-z\sqrt{(2\pi/\lambda)^2 + \frac{1}{l_c^2}}} \sin \left( \frac{2\pi x}{\lambda}\right) \label{eqn:interface_shape}
 \end{align}

\section{Micro force sensor}
